# Supplementary material for: MMInstruct: A High-Quality Multi-Modal Instruction Tuning Dataset with Extensive Diversity
Source: arXiv:2407.15838 source file (2024-08-07)
Supplement: Supplementary file 1 [file 6_appendix.tex]

% \begin{appendix}
% \section{image categories}

% \begin{itemize}
% \leftmargin 0.5cm
% \item image style
% \item image emotion
% \item object localization
% \item species recognition
% \item social relation
% \item attribute recognition
% \item meme comprehension
% \item complex reasoning
% \item landmark
% \item object relation
% \item commonsense reasoning
% \item posters
% \item brand recognition
% \item image quality
% \item future prediction
% \item image scene
% \item OCR
% \item artwork
% \item spatial relationship
% \item image comparison
% \end{itemize}
% \end{appendix}
